# Supplementary material for: Neural Multi-Quantile Forecasting for Optimal Inventory Management
Source: arXiv:2112.05673 source file (2021-12-10)
Supplement: Supplementary file 1 [file section_appendix_tables.tex]

\subsection{Tables}

In the following table $l_t$ denotes the series at time $t$, $b_t$ denotes the slope at time $t$, $s_t$ denotes the seasonal component of the series at time $t$ and $m$ denotes the season; $\alpha$, $\beta^*$, $\gamma$ and $\phi$ are smoothing parameters, $\phi_h = \sum_{i=1}^h \phi^i$ and $k$ is the integer part of $(h-1) / m$. 
This table shows recursive calculations and point forecasts.

\begin{landscape}
\begin{table}[htpb] 
\centering
\begin{tabular}{llll}
\toprule
\textbf{Trend} & \multicolumn{3}{c}{\textbf{Seasonal}} \\
& \textbf{None} & \textbf{Additive} & \textbf{Multiplicative} \\
\midrule
\textbf{N} & 
\shortstack[l]{$\hat{y}_{t+h|t} = l_t$ \\ $l_t = \alpha y_t + (1 - \alpha) l_{t-1}$} & 
\shortstack[l]{$\hat{y}_{t+h|t} = l_t + s_{t + h - m(k-1)}$ \\ $l_t = \alpha (y_t - s_{t-m}) + (1-\alpha) l_{t-1}$ \\ $s_t = \gamma(y_t - l_{t-1}) + (1 - \gamma)s_{t-m}$} & 
\shortstack[l]{$\hat{y}_{t+h|t} = l_t s_{t + h - m(k-1)}$ \\ $l_t = \alpha (y_t / s_{t-m}) + (1-\alpha) l_{t-1}$ \\ $s_t = \gamma(y_t / l_{t-1}) + (1 - \gamma)s_{t-m}$} \\
\hline
\textbf{A} & 
\shortstack[l]{$\hat{y}_{t+h|t} = l_t + hb_t$ \\ $l_t = \alpha y_t + (1 - \alpha)(l_{t-1} + b_{t-1})$ \\ $b_t = \beta^*(l_t - l_{t-1}) + (1 - \beta^*) b_{t-1}$} & 
\shortstack[l]{$\hat{y}_{t+h|t} = l_t + hb_t + s_{t+h-m(k-1)}$ \\ $l_t = \alpha (y_t - s_{t-m}) + (1 - \alpha)(l_{t-1} + b_{t-1})$ \\ $b_t = \beta^*(l_t - l_{t-1}) + (1 - \beta^*) b_{t-1}$ \\ $s_t = \gamma (y_t - l_{t-1} - b_{t-1}) + (1 - \gamma)s_{t-m}$} &
\shortstack[l]{$\hat{y}_{t+h|t} = (l_t + hb_t) s_{t+h-m(k-1)}$ \\ $l_t = \alpha (y_t/ s_{t-m}) + (1 - \alpha)(l_{t-1} + b_{t-1})$ \\ $b_t = \beta^*(l_t - l_{t-1}) + (1 - \beta^*) b_{t-1}$ \\ $s_t = \gamma (y_t / (l_{t-1} + b_{t-1})) + (1 - \gamma)s_{t-m}$} \\
\hline
\textbf{A$_d$} &
\shortstack[l]{$\hat{y}_{t+h|t} = l_t + \phi_h b_t$ \\ $l_t = \alpha y_t + (1 - \alpha)(l_{t-1} + \phi b_{t-1})$ \\ $b_t = \beta^*(l_t - l_{t-1}) + (1 - \beta^*) \phi b_{t-1}$} & 
\shortstack[l]{$\hat{y}_{t+h|t} = l_t + \phi_h b_t + s_{t+h-m(k-1)}$ \\ $l_t = \alpha (y_t - s_{t-m}) + (1 - \alpha)(l_{t-1} + \phi b_{t-1})$ \\ $b_t = \beta^*(l_t - l_{t-1}) + (1 - \beta^*) \phi b_{t-1}$ \\ $s_t = \gamma (y_t - l_{t-1} - \phi b_{t-1}) + (1 - \gamma)s_{t-m}$} &
\shortstack[l]{$\hat{y}_{t+h|t} = (l_t + \phi_h b_t) s_{t+h-m(k-1)}$ \\ $l_t = \alpha (y_t/ s_{t-m}) + (1 - \alpha)(l_{t-1} + \phi b_{t-1})$ \\ $b_t = \beta^*(l_t - l_{t-1}) + (1 - \beta^*) \phi b_{t-1}$ \\ $s_t = \gamma (y_t / (l_{t-1} + \phi b_{t-1})) + (1 - \gamma)s_{t-m}$} \\
\bottomrule
\end{tabular}
\caption{Recursive calculations and point forecasts for ETS models. N stands for None, A for Additive, A$_d$ for Additive damped and M for multiplicative.}
\label{table:state_space_models}
\end{table}
\end{landscape}
