# Supplementary material for: Neural Multi-Quantile Forecasting for Optimal Inventory Management
Source: arXiv:2112.05673 source file (2021-12-10)
Supplement: Supplementary file 2 [file section_appendix_data.tex]

\subsection{GLOBO Dataset}

\subsection{Barcel National Dataset}
