# Supplementary material for: Neural Multi-Quantile Forecasting for Optimal Inventory Management
Source: arXiv:2112.05673 source file (2021-12-10)
Supplement: Supplementary file 3 [file section_appendix_fformachallenges.tex]

\subsection{QFFORMA Ensemble Challenges}
