# Supplementary material for: Neural Multi-Quantile Forecasting for Optimal Inventory Management
Source: arXiv:2112.05673 source file (2021-12-10)
Supplement: Supplementary file 4 [file section_appendix_hyperparameters.tex]

\subsection{Hyperparameter Settings}
